# Supplementary material for: Disorder induced power-law response of a superconducting vortex on a plane
Source: arXiv:1401.0995 ancillary file (2014-01-06)
Supplement: Supplementary file 1 [file Supplemental_Material.pdf]

# Disorder induced power-law response of a superconducting vortex on a plane: Supplemental Material

N. Shapira, Y. Lamhot, O. Shpielberg, Y. Kafri, B. J. Ramshaw, D. A. Bonn, Ruixing Liang, W. N. Hardy, O. M. Auslaender

## 1. The transition temperature $T_c$ and Meissner repulsion

We determined the superconducting transition temperature of our sample $T_c$ from the disappearance of the diamagnetic Meissner response. In the superconducting state a Meissner levitation force acts on the magnetic tip [1]. The gradient of this repulsive force is accompanied by a frequency shift $\Delta f$ of the cantilever resonance [2]:

$$\Delta f = -\frac{f_0}{2k}\frac{\partial F_z}{\partial z} = \frac{f_0}{2k}\frac{\mu_0 \tilde{m}^2}{4\pi}\left[\frac{1}{z+\lambda_{ab}} + \frac{h_0}{\left(z+\lambda\right)^2_{ab}} + \frac{h_0^2}{2\left(z+\lambda\right)^3_{ab}}\right] \qquad (1)$$

Here $f_0$ and $k$ are the free-space resonant frequency and spring constant of the cantilever, $\mu_0$ is the vacuum permeability and $\tilde{m}$ and $h_0$ the magnetization per unit area and truncation length of the MFM tip (see Supplemental Material - The force formula).

We performed a series of touch-downs (approaching the MFM tip towards the sample surface by reducing $z$ while recording $\Delta f$ ). Supplementary Fig. 1 shows three of these touch-downs at temperatures $78K$, $90K$ and $92K$. The very pronounced frequency shift which grows as we approach the sample at lower temperatures vanishes between $90K$ and $92K$ and allows us to determine that $T_c \approx 91K$ with an accuracy of $1K$.

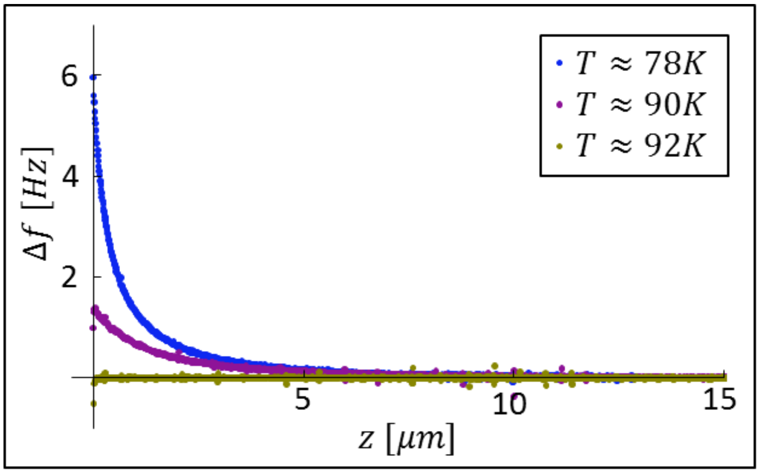


Supplementary Figure 1: Meissner response curves obtained from touch-downs at temperatures $78K$, $90K$ and $92K$. All curves were obtained with the same MFM tip in the same run.

**2. The force formula**

The transverse force resulting from the magnetic interaction between the magnetic field of a vortex $\vec{B}_{vor}(\vec{r})$ and the magnetic layer coating the MFM tip [specific magnetization $\vec{M}_{tip}(\vec{r})$] is equal to

$$F_\rho = -\partial_\rho \int \vec{M}_{tip} \cdot \vec{B}_{vor} dV . \qquad (2)$$

We model the tip as a sharp, single-domain, conical shell truncated at a distance $h_0 \approx 250nm$ from the apex (cf. SFig. 3) and further simplify our calculations by projecting the cone geometry on the cone axis, i.e. $\vec{M}_{tip}(\vec{r}) = \tilde{m}(z-h_0)\Theta(z-z_{tip})\hat{z}$ where $\tilde{m} \approx 0.2A$ is the magnetization per unit area we obtain from fits of Meissner response touchdowns to Supplemental Eq. 1 and $\Theta(z)$ is the Heaviside step function. In addition we use a $z \gg \lambda_{ab}$ approximation for the magnetic field from a single vortex [3]:

$$\vec{B}_{vor}(r) = \frac{\Phi_0}{2\pi} \frac{\rho\hat{\rho} + (z+\lambda_{ab})\hat{z}}{\left[\rho^2 + (z+\lambda_{ab})^2\right]^{3/2}} \qquad (3)$$

where $\Phi_0 = h/2e \approx 2.07 \times 10^{-15} Tm^2$ is the flux quantum ($h$ is the Planck constant and $e$ is the magnitude of the electron charge). This leads to the expression we use to approximate the force exerted on the vortex right before each jump:

$$F_\rho = \frac{\Phi_0 \tilde{m}}{2\pi} \frac{h_0\rho^2 + \left[\rho^2 + (z+\lambda_{ab})^2\left(\sqrt{\rho^2+(z+\lambda_{ab})^2} - z - \lambda_{ab}\right)\right]}{\rho\left[\rho^2+(z+\lambda_{ab})^2\right]^{3/2}} . \qquad (4)$$

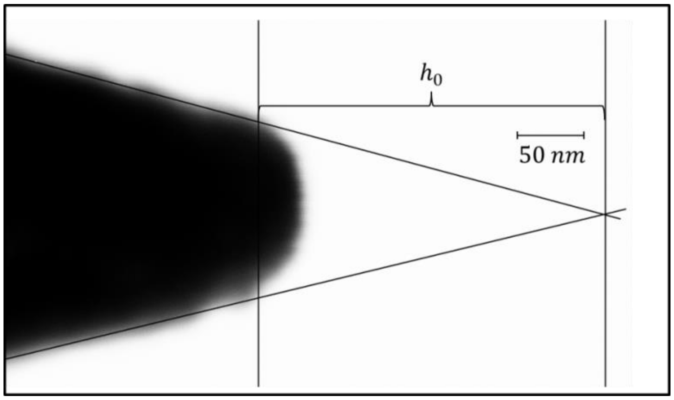


Supplementary Figure 2: Scanning electron microscopy (SEM) scan of the sharp end of the MFM tip that measured all vortex jumps in this work.

### 3. The jump detection algorithm

We extracted the sizes of the vortex jumps with the aid of a "jump extraction algorithm". The algorithm is designed to distinguish between the sharp discontinuities of the signal and measurement noise. It works as follows:

a. Finding candidate jumps
   For each line-scan we find all local maxima below a given maximal value $\Delta f^{\max}$. For example, the maximal $\Delta f$ threshold in Figs. 2a,2b (main text) is $\Delta f^{\max} = -0.25Hz$.
b. Approximating a static vortex
   We remove all the local maxima found in (a) by cutting out the "valleys" – all data points between each local maximum ( $x_{jump}$ ) and the first point on the nearby slope with the same $\Delta f$ value as the local maximum ( $x^*$ ). After completing this step we obtain a signal which is an estimate of the signal from a completely pinned (non-jumping) static vortex.
c. Derivative test
   We fit a Gaussian to the static vortex signal from (b) to help distinguish between real jumps and noise. Since the signature of a jump is a discontinuity of the signal right after the jump, we return to the original data and look for local maxima below $\Delta f^{\max}$ that also have a derivative larger than the derivative of the Gaussian at the same $\Delta f$ value. We identify these local maxima as those that resulted from vortex jumps.
d. Retrieving the jump sizes
   We again remove valleys but this time we do so only for the local maxima found in (c). The lengths of the segments between each local maximum and the corresponding point on the nearby slope are our jump sizes, i.e. $\Delta_{jump} = \left| x_{jump} - x^* \right|$. We record $\Delta_{jump}$ along with the relative position of the jump $x_{jump}$ and the value of $\Delta f$ at the jump.
e. Retrieving the force
   From the values of $\Delta f$ we obtain in (d) we calculate the values of the force along the TB
   $F_x = F_\rho \cos(\theta) = \left( x_{jump} / \rho_v \right) F_\rho$   $F_x = F_\rho cos(\theta) = (x/\rho_v)F_\rho$.

The error on the extracted jump length $\approx 1nm$ and the efficiency of jump detection is $\approx 90\%$.

## 4. Self-averaging of tilted vortices

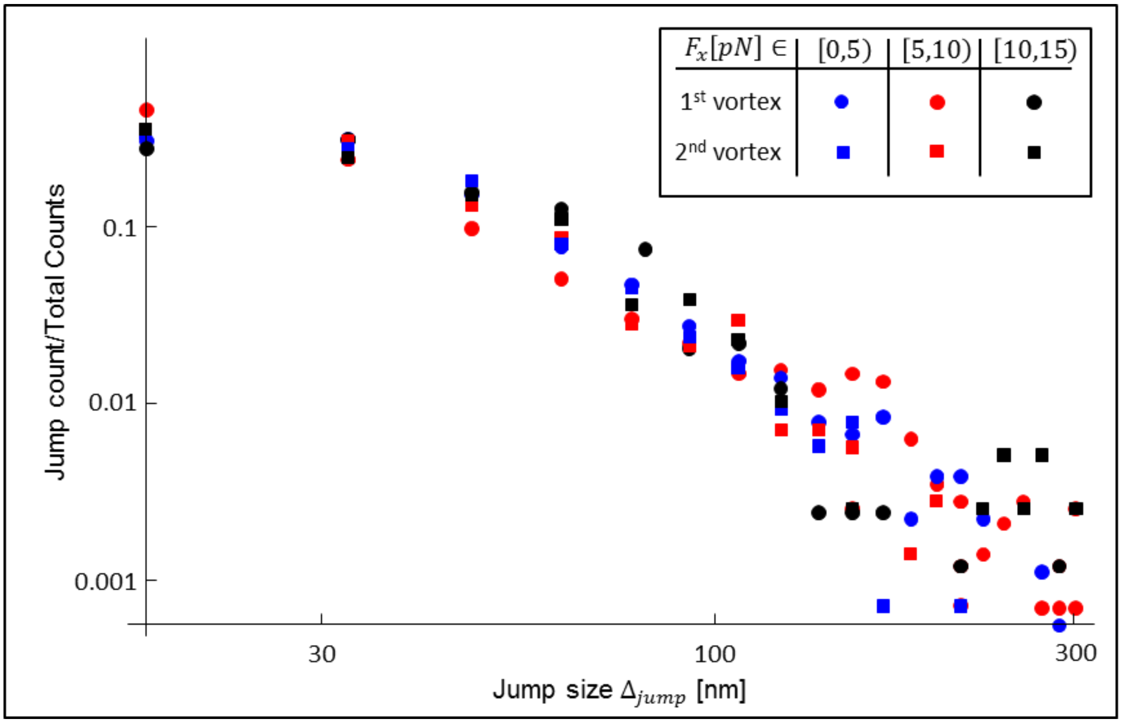


Supplementary Figure 3: Normalized jump length distributions measured for the two widely separated TB vortices discussed in the main text for different force ranges. The statistically similar distributions confirm that even for each vortex separately the distribution does not depend on the force.

## 5. Minimum tilt for self-averaging

For sufficient tilt a vortex samples an effectively new energy landscape and therefore one can obtain disorder averages from measurements on a single vortex. According to the theory of DPRM [4] the tilt is sufficient if the applied force is much larger than $F_{\min} = \kappa \left( L/a_z \right)^{\zeta - 1}$. In our experiment $F_{\min} \approx 0.15 pN$, a scale much lower than the typical forces we apply on vortices with the MFM tip.

## 6. Force independent self-averaging of tilted vortices

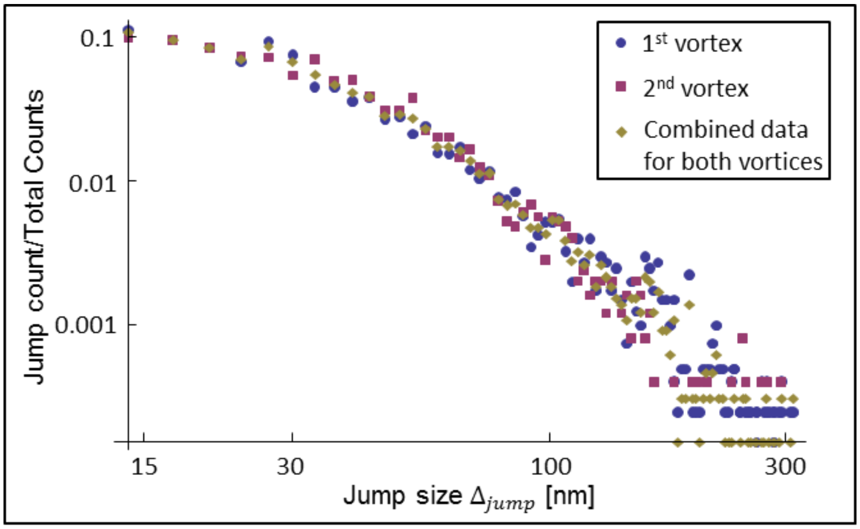


Supplementary Figure 4: Double logarithmic plot of the normalized jump length distributions measured for two widely separated and isolated vortices trapped on the TB alongside the normalized jump length distribution for both vortices together. The collapse of the distributions onto each other implies that we could have obtained disorder-averaged quantities even from measurements on a single vortex.

## 7. The line tension $\kappa$

The line tension of a vortex in a superconducting material characterized by an anisotropy parameter $\varepsilon$ is given by [4]:

$$\kappa = \frac{\Phi_0^2}{4\pi\mu_0}\left(\frac{\varepsilon}{\lambda_{ab}}\right)^2. \quad (5)$$

## References


1. Kogan, V. G. Meissner response of anisotropic superconductors. *Phys. Rev. B* **68,** 104511 (2003).
2. Luan, L. *et al.* Local measurement of the penetration depth in the pnictide superconductor $Ba(Fe_{0.95}Co_{0.05})_2As_2$. *Phys. Rev. B* **81,** 100501 (2010).
3. Pearl, J. Structure of Superconductive Vortices near a Metal-Air Interface. *J. Appl. Phys.* **37,** 4139–4141 (1966).
4. Hwa, T. & Fisher, D. S. Anomalous fluctuations of directed polymers in random media. *Phys. Rev. B* **49,** 3136–3154 (1994).
